# Supplementary material for: Online Reasoning Video Segmentation with Just-in-Time Digital Twins
Source: arXiv:2503.21056 source file (2025-03-27)
Supplement: Supplementary file 1 [file appendix.tex]

\appendix

% examples for graph (varying depth/width)
System: You are an expert in computer vision and reasoning. Analyze the query to select required vision models.

Query: [Input Query Text]

Required Analysis:
1. Identify semantic requirements (object categories, attributes)
2. Detect spatial relationships (relative positions, distances)
3. Recognize temporal dependencies (motion, events, ordering)

Output Format:
{
    "models": {
        "model_name": {
            "purpose": "specific task",
            "justification": "reasoning for selection"
        }
    },
    "dependencies": [ordered list of execution requirements]
}

For example, given the query ``\textit{segment objects that moved behind the dining table after the person sat down}'', the planner identifies:
